# Supplementary material for: AdaGaR: Adaptive Gabor Representation for Dynamic Scene Reconstruction
Source: arXiv:2601.00796 source file (2026-01-02)
Supplement: Supplementary file 1 [file _supplementary.tex]

\input{_constants}
\review % \review OR \cameraready

\documentclass[10pt,twocolumn,letterpaper]{article}
\input{cvpr_header}
\myexternaldocument{_main}
\begin{document}

%% TITLE
\title{\paperTitle}
\author{\authorBlock}
\maketitlesupplementary

\appendix
\input{12_appendix}

{\small
\bibliographystyle{ieeenat_fullname}
\bibliography{11_references}
}

\end{document}
